# Supplementary material for: RECOVAR: Representation Covariances on Deep Latent Spaces for Seismic Event Detection
Source: arXiv:2407.18402 source file (2026-11-14)
Supplement: Supplementary file 1 [file si.tex]

%%%%%%%%%%%%%%%%%%%%%%%%%%%%%%%%%%%%%%%%%%%%%%%%%%%%%%%%%%%%%%%%%%%%%%%%%%%%
% AGUtmpl.tex: this template file is for articles formatted with LaTeX2e,
% Modified December 2018
%
% This template includes commands and instructions
% given in the order necessary to produce a final output that will
% satisfy AGU requirements.
%
% FOR FIGURES, DO NOT USE \psfrag
%
%%%%%%%%%%%%%%%%%%%%%%%%%%%%%%%%%%%%%%%%%%%%%%%%%%%%%%%%%%%%%%%%%%%%%%%%%%%%
%
% IMPORTANT NOTE:
%
% SUPPORTING INFORMATION DOCUMENTATION IS NOT COPYEDITED BEFORE PUBLICATION.
%
%
%
%%%%%%%%%%%%%%%%%%%%%%%%%%%%%%%%%%%%%%%%%%%%%%%%%%%%%%%%%%%%%%%%%%%%%%%%%%%%
%
% Step 1: Set the \documentclass
%
%
% PLEASE USE THE DRAFT OPTION TO SUBMIT YOUR PAPERS.
% The draft option produces double spaced output.
%
% Choose the journal abbreviation for the journal you are
% submitting to:

% jgrga JOURNAL OF GEOPHYSICAL RESEARCH (use for all of them)
% gbc   GLOBAL BIOCHEMICAL CYCLES
% grl   GEOPHYSICAL RESEARCH LETTERS
% pal   PALEOCEANOGRAPHY
% ras   RADIO SCIENCE
% rog   REVIEWS OF GEOPHYSICS
% tec   TECTONICS
% wrr   WATER RESOURCES RESEARCH
% gc    GEOCHEMISTRY, GEOPHYSICS, GEOSYSTEMS
% sw    SPACE WEATHER
% ms    JAMES
% ef    EARTH'S FUTURE
%
%
%
% (If you are submitting to a journal other than jgrga,
% substitute the initials of the journal for "jgrga" below.)

\documentclass[draft,jgrga]{agutexSI2019}

% Fix for infinite shrinkage error.
\makeatletter
\def\@makecol{\setbox\@outputbox
     \vbox{\boxmaxdepth \maxdepth
\ifdim\ht\dbltopins<1pt\else\unvbox\dbltopins\fi
     \unvbox\@cclv
\ifdim\ht\dblbotins<1pt\else\unvbox\dblbotins\fi%
\ifvoid\footins\else\vskip\skip\footins\footnoterule\unvbox\footins\fi
%\vss
\vskip 0pt plus 1fil minus \maxdimen
}%
%\global\savefigandtabnumber\figandtabnumber
%\global\advance\savefigandtabnumber by 1 %% Because loop stops one short
                                         %% of the total number of figs
\global\savedblfigandtabnumber\dblfigandtabnumber
   \xdef\@freelist{\@freelist\@midlist}\gdef\@midlist{}\@combinefloats
   \setbox\@outputbox\vbox to\@colht{\boxmaxdepth\maxdepth
   \@texttop\dimen128=\dp\@outputbox\unvbox\@outputbox
   \vskip-\dimen128\@textbottom}%
   \global\maxdepth\@maxdepth}
\makeatother

 \usepackage{graphicx}
 \usepackage{amssymb}
 \usepackage{amsmath}
%
%  Uncomment the following command to allow illustrations to print
%   when using Draft:
\setkeys{Gin}{draft=false}
%
% You may need to use one of these options for graphicx depending on the driver program you are using. 
%
% [xdvi], [dvipdf], [dvipsone], [dviwindo], [emtex], [dviwin],
% [pctexps],  [pctexwin],  [pctexhp],  [pctex32], [truetex], [tcidvi],
% [oztex], [textures]
%
%
%% ------------------------------------------------------------------------ %%
%
%  ENTER PREAMBLE
%
%% ------------------------------------------------------------------------ %%

% Author names in capital letters:
%\authorrunninghead{BALES ET AL.}

% Shorter version of title entered in capital letters:
%\titlerunninghead{SHORT TITLE}

%Corresponding author mailing address and e-mail address:
%\authoraddr{Corresponding author: A. B. Smith,
%Department of Hydrology and Water Resources, University of
%Arizona, Harshbarger Building 11, Tucson, AZ 85721, USA.
%(a.b.smith@hwr.arizona.edu)}

\begin{document}

%% ------------------------------------------------------------------------ %%
%
%  TITLE
%
%% ------------------------------------------------------------------------ %%

%\includegraphics{agu_pubart-white_reduced.eps}

\title{RECOVAR: Representation Covariances on Deep Latent Spaces for Seismic Event Detection}
%
% e.g., \title{Supporting Information for "Terrestrial ring current:
% Origin, formation, and decay $\alpha\beta\Gamma\Delta$"}
%
%DOI: 10.1002/%insert paper number here%

%% ------------------------------------------------------------------------ %%
%
%  AUTHORS AND AFFILIATIONS
%
%% ------------------------------------------------------------------------ %%

% List authors by first name or initial followed by last name and
% separated by commas. Use \affil{} to number affiliations, and
% \thanks{} for author notes.
% Additional author notes should be indicated with \thanks{} (for
% example, for current addresses).

% Example: \authors{A. B. Author\affil{1}\thanks{Current address, Antartica}, B. C. Author\affil{2,3}, and D. E.
% Author\affil{3,4}\thanks{Also funded by Monsanto.}}

\authors{O. Efe \affil{1}, A. Ozakin \affil{1}}

% \affiliation{1}{First Affiliation}
% \affiliation{2}{Second Affiliation}
% \affiliation{3}{Third Affiliation}
% \affiliation{4}{Fourth Affiliation}

\affiliation{1}{Department of Physics, Bogazici University, Istanbul}
%(repeat as many times as is necessary)

%% ------------------------------------------------------------------------ %%
%
%  BEGIN ARTICLE
%
%% ------------------------------------------------------------------------ %%

% The body of the article must start with a \begin{article} command
%
% \end{article} must follow the references section, before the figures
%  and tables.

\begin{article}

%% ------------------------------------------------------------------------ %%
%
%  TEXT
%
%% ------------------------------------------------------------------------ %%

\noindent\textbf{Contents of this file}
%%%Remove or add items as needed%%%
\begin{enumerate}
\item Text S1 to S9
\item Figures S1 to S4
\end{enumerate}

\noindent\textbf{Introduction}
This supporting document involves the details of the layers used in the Autoencoder, 
possible ways to extract classification information from representations, information on datasets, and training and testing details. 
For more information on the architecture of the Autoencoder, refer to Text S1. 
Different ways of extracting a measure of signal content in a waveform involve computing 
the autocovariance of a latent representation, or cross-covariances between pairs of representations. The details of the different approaches are given in Text S2, S3, S4.
The properties of the datasets used are shared in detail in Text S5, while the preprocessing procedures applied during training and testing are shared in Text S6 and S7, respectively. Selected hyperparameters, training procedures, and observations can be found in Text S8 and S9.

\noindent\textbf{Text S1} \emph{Building blocks of CNN Autoencoder}.
The \emph{Downsampling layers} in Figure \ref{fig:cnn_autoencoder_building_blocks} consist of reflective padding, followed by a 1-dimensional convolution with stride 2 and batch normalization, and have ReLU activation. Due to the stride, the output length of a Downsampling layer along the time direction is half its input length.  Five Downsampling layers with convolutional window sizes 15, 13, 11, 9, 7 and output channel (filter) counts 8, 16, 32, 64, 64 are used in succession, which reduces the length of input waveforms along the time axis from 3000 to 94 while increasing the number of channels from 3 to 64. Since some of the output lengths are not divisible by 2,
we use a  separate  ``reflect padding'' layer to make
the lengths compatible between  Downsampling layers. 

The \emph{Residual layers} in Figure \ref{fig:cnn_autoencoder_building_blocks} do not change the dimensions of their input, but aim to further improve the representation by utilizing two identical stacks containing 1D 
Convolution, Batch Normalization, and ReLU Activation layers. We add 
a residual (``skip'') connection around these stacks that adds
the input to the Residual layer to the output of the second stack. This sum is then passed through a ReLU activation to form the output. We use five of these Residual layers with 64 filter and filter window size 5. The last Residual layer uses linear activation instead of ReLU.

The \emph{Upsampling layers} in Figure \ref{fig:cnn_autoencoder_building_blocks} are connected to the output of last Residual layer. Series of Upsampling layers form the decoder structure. These layers consist of plain upsampling followed by padding, 1-dimensional convolution, batch normalization, and a ReLU activation. Five such upsampling layers with convolutional window sizes 7, 9, 11, 13, 15 and filter counts 32, 16, 8, 4, and 3 are used to increase the length of the waveform representations along the time axis from 94 to 3000 while decreasing the number of channels from 64 to 3. Dually to the Downsampling case, each Upsampling layer doubles the temporal length of its output. Once again, to ensure shape compatibility of the final decoded output with the original waveform input, we use a cropping layer.

\noindent\textbf{Text S2} \emph{Details for single autoencoder method}.
In this simple approach, we compute the autocovariance of each channel and then average the resulting multichannel signal over channels. We observe that, contrary to noise waveforms, earthquake representations obtained by training an autoencoder tend to be composed of more long-term features. This results in the autocovariance of noise samples having a narrow spike at \(\text{lag}=0\), while for earthquake signals, we obtain a wider and smoother peak \ref{fig:autcovariance_samples}. This is due to the larger amount of coherence and shared information between different timesteps for earthquake samples compared to noise, which allows us to use it as a detection mechanism. 

\noindent\textbf{Text S3} \emph{Details for Augmented autoencoder method}.
We apply random augmentations to raw waveforms and then take the cross-covariances of their latent representations obtained by using the identical autoencoders for each augmented waveform. The method has similarities to Self-Supervised Learning (SSL)~\cite{con:liu2021self}, which uses augmentations to obtain robust representations for classification purposes. 

The intuitive motivation for this approach is that
earthquake waveforms are expected to be composed of  
robust features, so small changes in the raw waveform 
shouldn't significantly alter their latent representations. 
As a result, the cross-covariance of the latent 
representations of two augmented waveforms is
expected to give a more robust peak than
what gets for a noise waveform and its augmentations. 

We have observed that using an ensemble of augmentations
and computing the average of the pairwise cross-covariances (instead of just using two augmentations) improves stability and performance.

As for the specific augmentation technique to use, we
tried some of the standard time series data 
augmentation techniques~\cite{wen2020time}  such as
simple additive noise and phase warping (adding random 
phase in the frequency domain), and our experiments
have shown that time-warping augmentation
performs well and gives more stable results compared to other methods. 

Time warping is accomplished by remapping the time axis of the original waveform by a monotonically
increasing function. The relevant function is obtained by selecting random deviations from the actual time at certain ``knots'' and interpolating between the knots with the BSpline algorithm and discretizing. We sample \(4\) knots from a zero-mean Gaussian distribution with standard deviation \(0.15\). Refer to ~\cite{wen2020time} for more details.

\noindent\textbf{Text S4} \emph{Details of Multiple autoencoders method}.
We used an ensemble of encoder-decoder structures to obtain multiple representations of a single waveform. The idea is similar to the augmentation-based method in that, once the autoencoders are trained, we compute the average of the pairwise cross-covariances of different autoencoder representations (instead of different augmentations).

An important point is that this approach also affects the training phase. Since a multitude of autoencoders can learn completely different representations, computing the pairwise covariances of otherwise unconstrained autoencoders may not be an effective way to detect signals. To make the outputs of the autoencoders comparable, we also learn an additional set of linear ``projection'' matrices at the output of each autoencoder. The projection
matrices are trained to maximize the similarities between the corresponding channels of different autoencoders.

More explicitly, we simultaneously train the projection matrices and the autoencoders, but as before, the gradient updates of the autoencoders only use the reconstruction loss to allow different autoencoders to learn different representations, while the gradient updates for the projection matrices use another RMS loss as described below, to map the outputs of different autoencoders to each other.

Let \(h^e \in \mathbb{R}^{N_L \times C_L}\) denote the projected latent representation of the \(e\)'th member of the ensemble, where \(N_L\) and \(C_L\) are latent numbers of timesteps and channels, respectively. Before calculating the loss for training the projection matrices, each channel \(c \in [0, C_L - 1]\) is centered on \(\sum_n h^e_{nc} = 0\) and normalized to unit variance. The projection loss \(L_{proj}\) is then calculated as the RMS difference between pairs of projected representations, the mean being taken over all pairs, channels, and time steps.

We emphasize that the gradient updates of the projection matrices and the autoencoder layers are made concerning different losses, to allow the system to learn different representations while also learning to relate them to each other. 

\noindent\textbf{Text S5} \emph{Description of datasets}.
Both datasets utilize three channels—East (E), North (N), and Vertical (Z)—and maintain a consistent sampling rate of 100 Hz. In terms of data volume, INSTANCE surpasses STEAD with 1,159,249 earthquake waveforms compared to STEAD's 1,050,000, and it also includes a greater number of noise waveforms, numbering 132,330 versus STEAD's 100,000. Additionally, INSTANCE features longer time windows of 120 seconds, double that of STEAD's 60 seconds, and extends the epicentral distance coverage up to
600 kilometers, whereas STEAD is limited to distances below 350 kilometers. Geographically, STEAD offers a global perspective, while INSTANCE is focused specifically on the region of Italy.

\noindent\textbf{Text S6} \emph{Preprocessing for training}.
To form the training set, we follow the procedure
described in~\cite{rev:munchmeyer2022picker,rev:woollam2022seisbench}
to randomly crop \(2/3\) of the earthquake waveforms in a way that guarantees to have at least one phase arrival within the window, and we randomly cropped the remaining earthquake waveforms and all of the noise waveforms without any such constraint.

\noindent\textbf{Text S7} \emph{Testing procedure}.
In the testing phase, following~\cite{rev:munchmeyer2022picker,rev:woollam2022seisbench}, 
we cropped the earthquake waveforms in a way that guarantees that the onset time is inside the window with a \(3\) second margin. As in~\cite{rev:munchmeyer2022picker}, we used
\(60\%\) of the whole data set for training, however, to get a more robust measure of test performance, we used 5-fold cross-validation at the test phase instead of using a single hold-out. Thus, instead of the \(10\%\) validation and \(30\%\) test size used in~\cite{rev:munchmeyer2022picker, rev:woollam2022seisbench}, we used \(20\%\) for both.

\noindent\textbf{Text S8} \emph{Optimization}.
We have used the ADAM optimizer with a constant learning rate of \(10^{-4}\) and \(\epsilon=10^{-7}\). We selected filter coefficients \(\beta_1\) and \(\beta_2\) as \(0.99\) and \(0.999\), respectively. We kept other settings in their default values, in particular, we didn't use additional exponential moving average filtering, weight decay, 
or gradient clipping.

\noindent\textbf{Text S9} \emph{Computational resouces and time}.
Training is carried out on a workstation with a single NVIDIA GTX3090TI GPU. Training the CNN autoencoder took \(1.5\) minutes per epoch on the preprocessed version of the INSTANCE dataset and \(1.25\) minutes on the preprocessed version of the STEAD dataset. Training the ``ensemble of autoencoders'' for a single epoch took \(7.5\) minutes for INSTANCE and \(6.5\) minutes for STEAD. Since we used preprocessed data, a negligible amount of time was spent on data generation. 

\bibliography{biblio} 

%% ------------------------------------------------------------------------ %%
%
%  END ARTICLE
%
%% ------------------------------------------------------------------------ %%
\end{article}

\clearpage

\begin{figure}[t]
    \centering
    \setfigurenum{S1}
    \noindent\includegraphics[width=\textwidth]{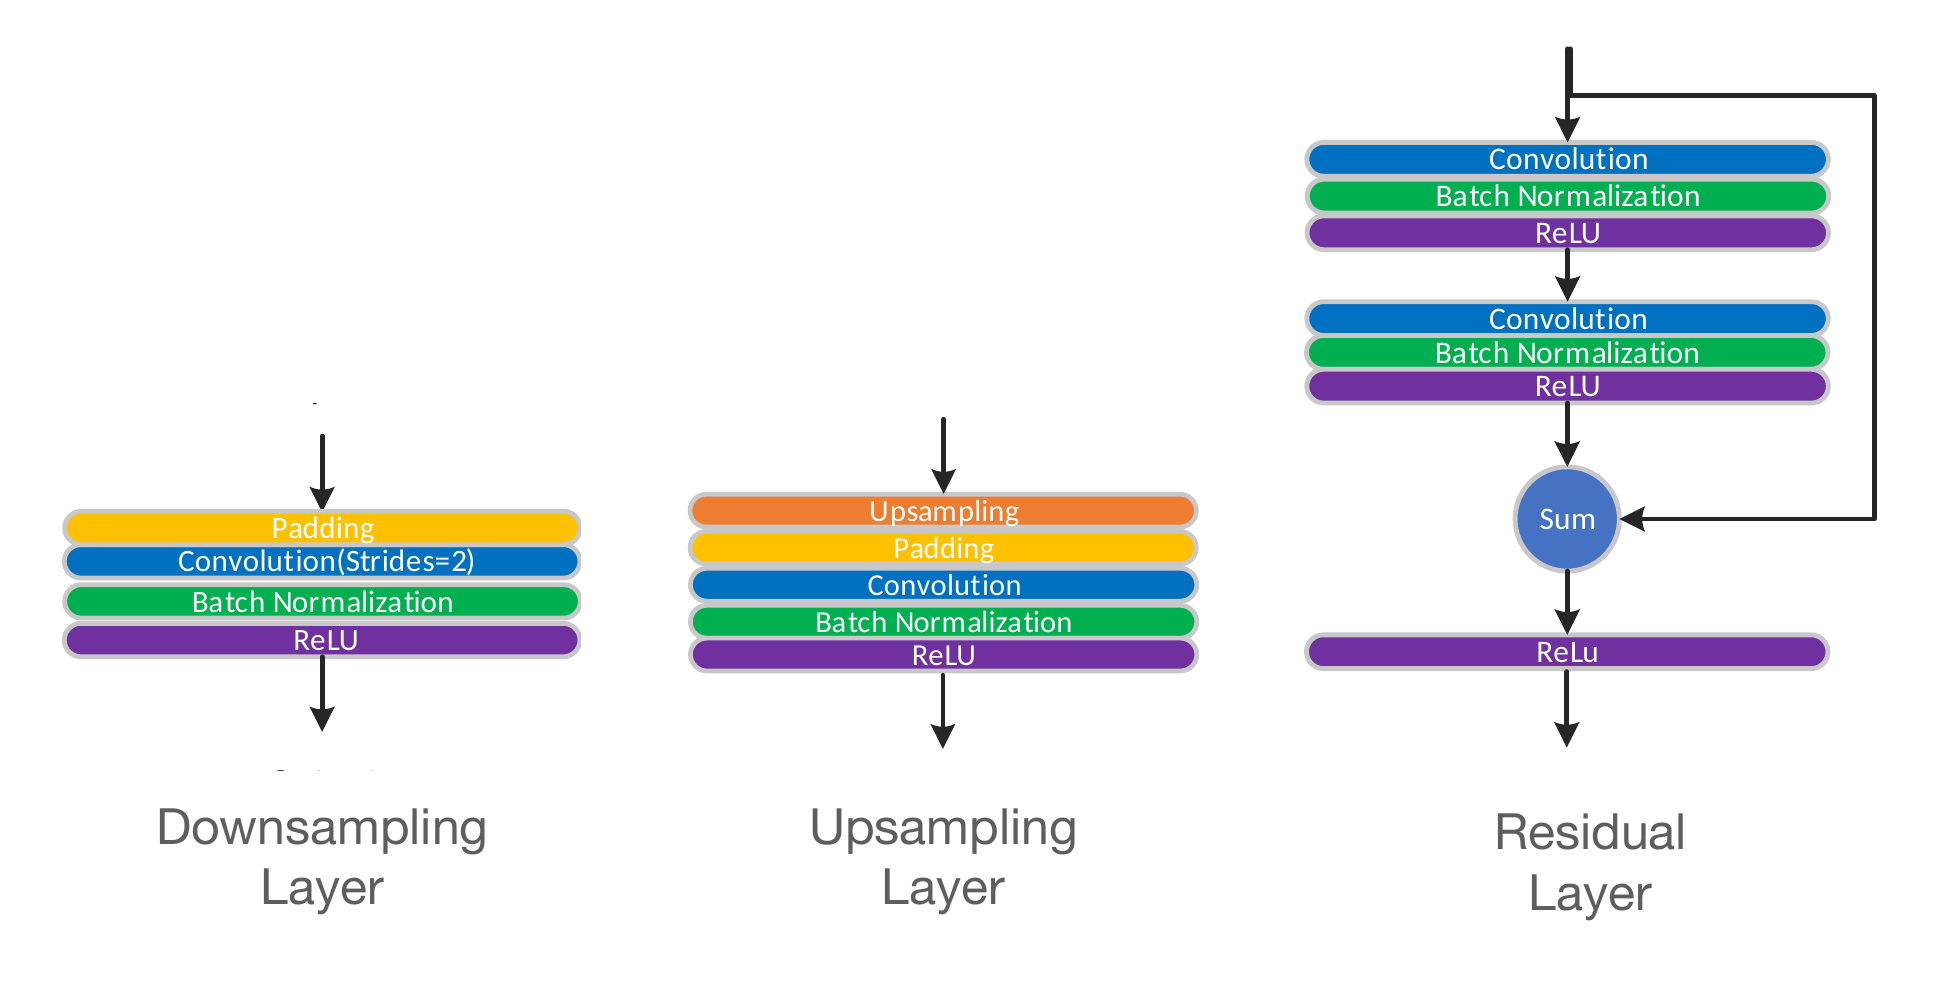}
    \caption{Building blocks of CNN Autoencoder.}
    \label{fig:cnn_autoencoder_building_blocks}
\end{figure}

\begin{figure}[t]\label{representation_mutual_info}
    \centering
    \setfigurenum{S2}
    \noindent\includegraphics[width=0.8\textwidth]{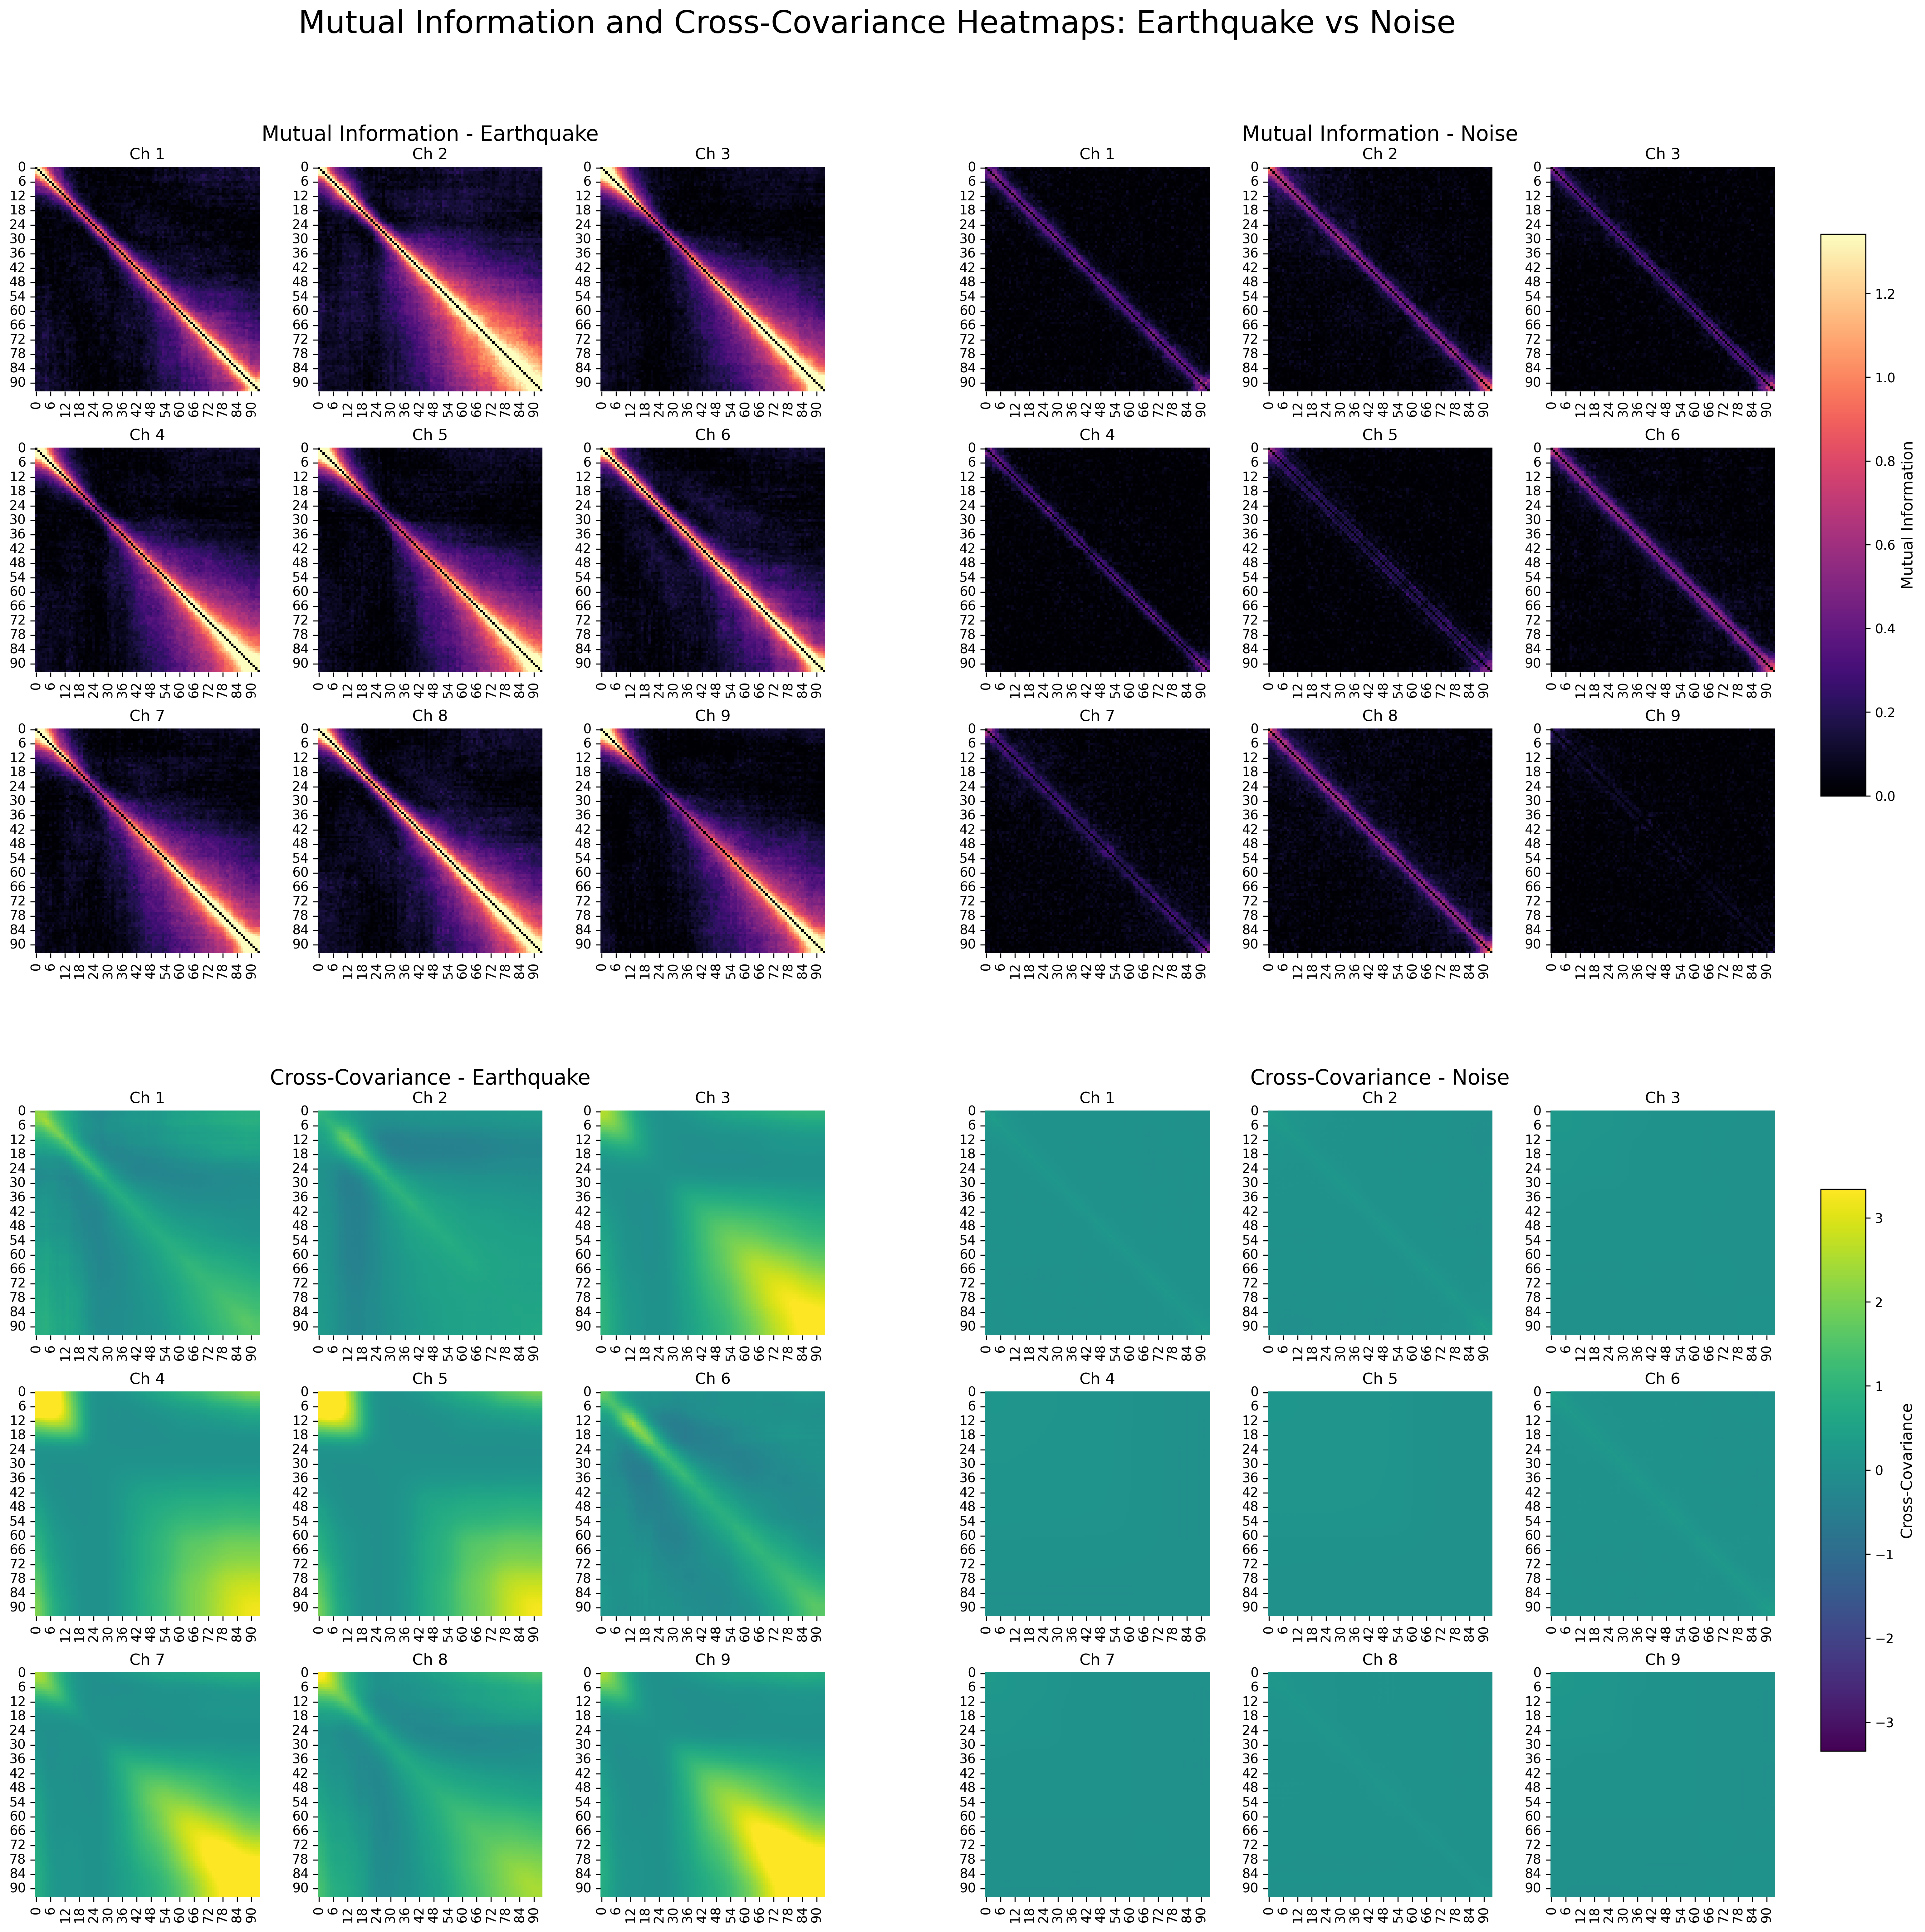}
    \caption{Heatmaps of Mutual information and Cross-covariances between timestep pairs for 9 randomly selected latent space channels. Horizontal and vertial axis of the heatmaps correspond to timestep indices. The top-left 3x3 figures show the mutual information profiles for a set of earthquake signals. The brighter color of the plots near the diagonal indicates strong shared information between close timesteps. However, for a set of noise signals (shown on the top-right 3x3 figures), we see that the shared information is almost zero except for very close timesteps. In the bottom figures, we show
    similar plots for cross-covariance profiles instead of mutual information. This behavior justifies the intuition mentioned in the paper on why using the cross-covariance in the latent space can be sufficient for detecting earthquake and noise waveforms.}
    \label{fig:mutual_info}
\end{figure}

\begin{figure}[t]
    \centering
    \setfigurenum{S3}
    \noindent\includegraphics[width=\linewidth]{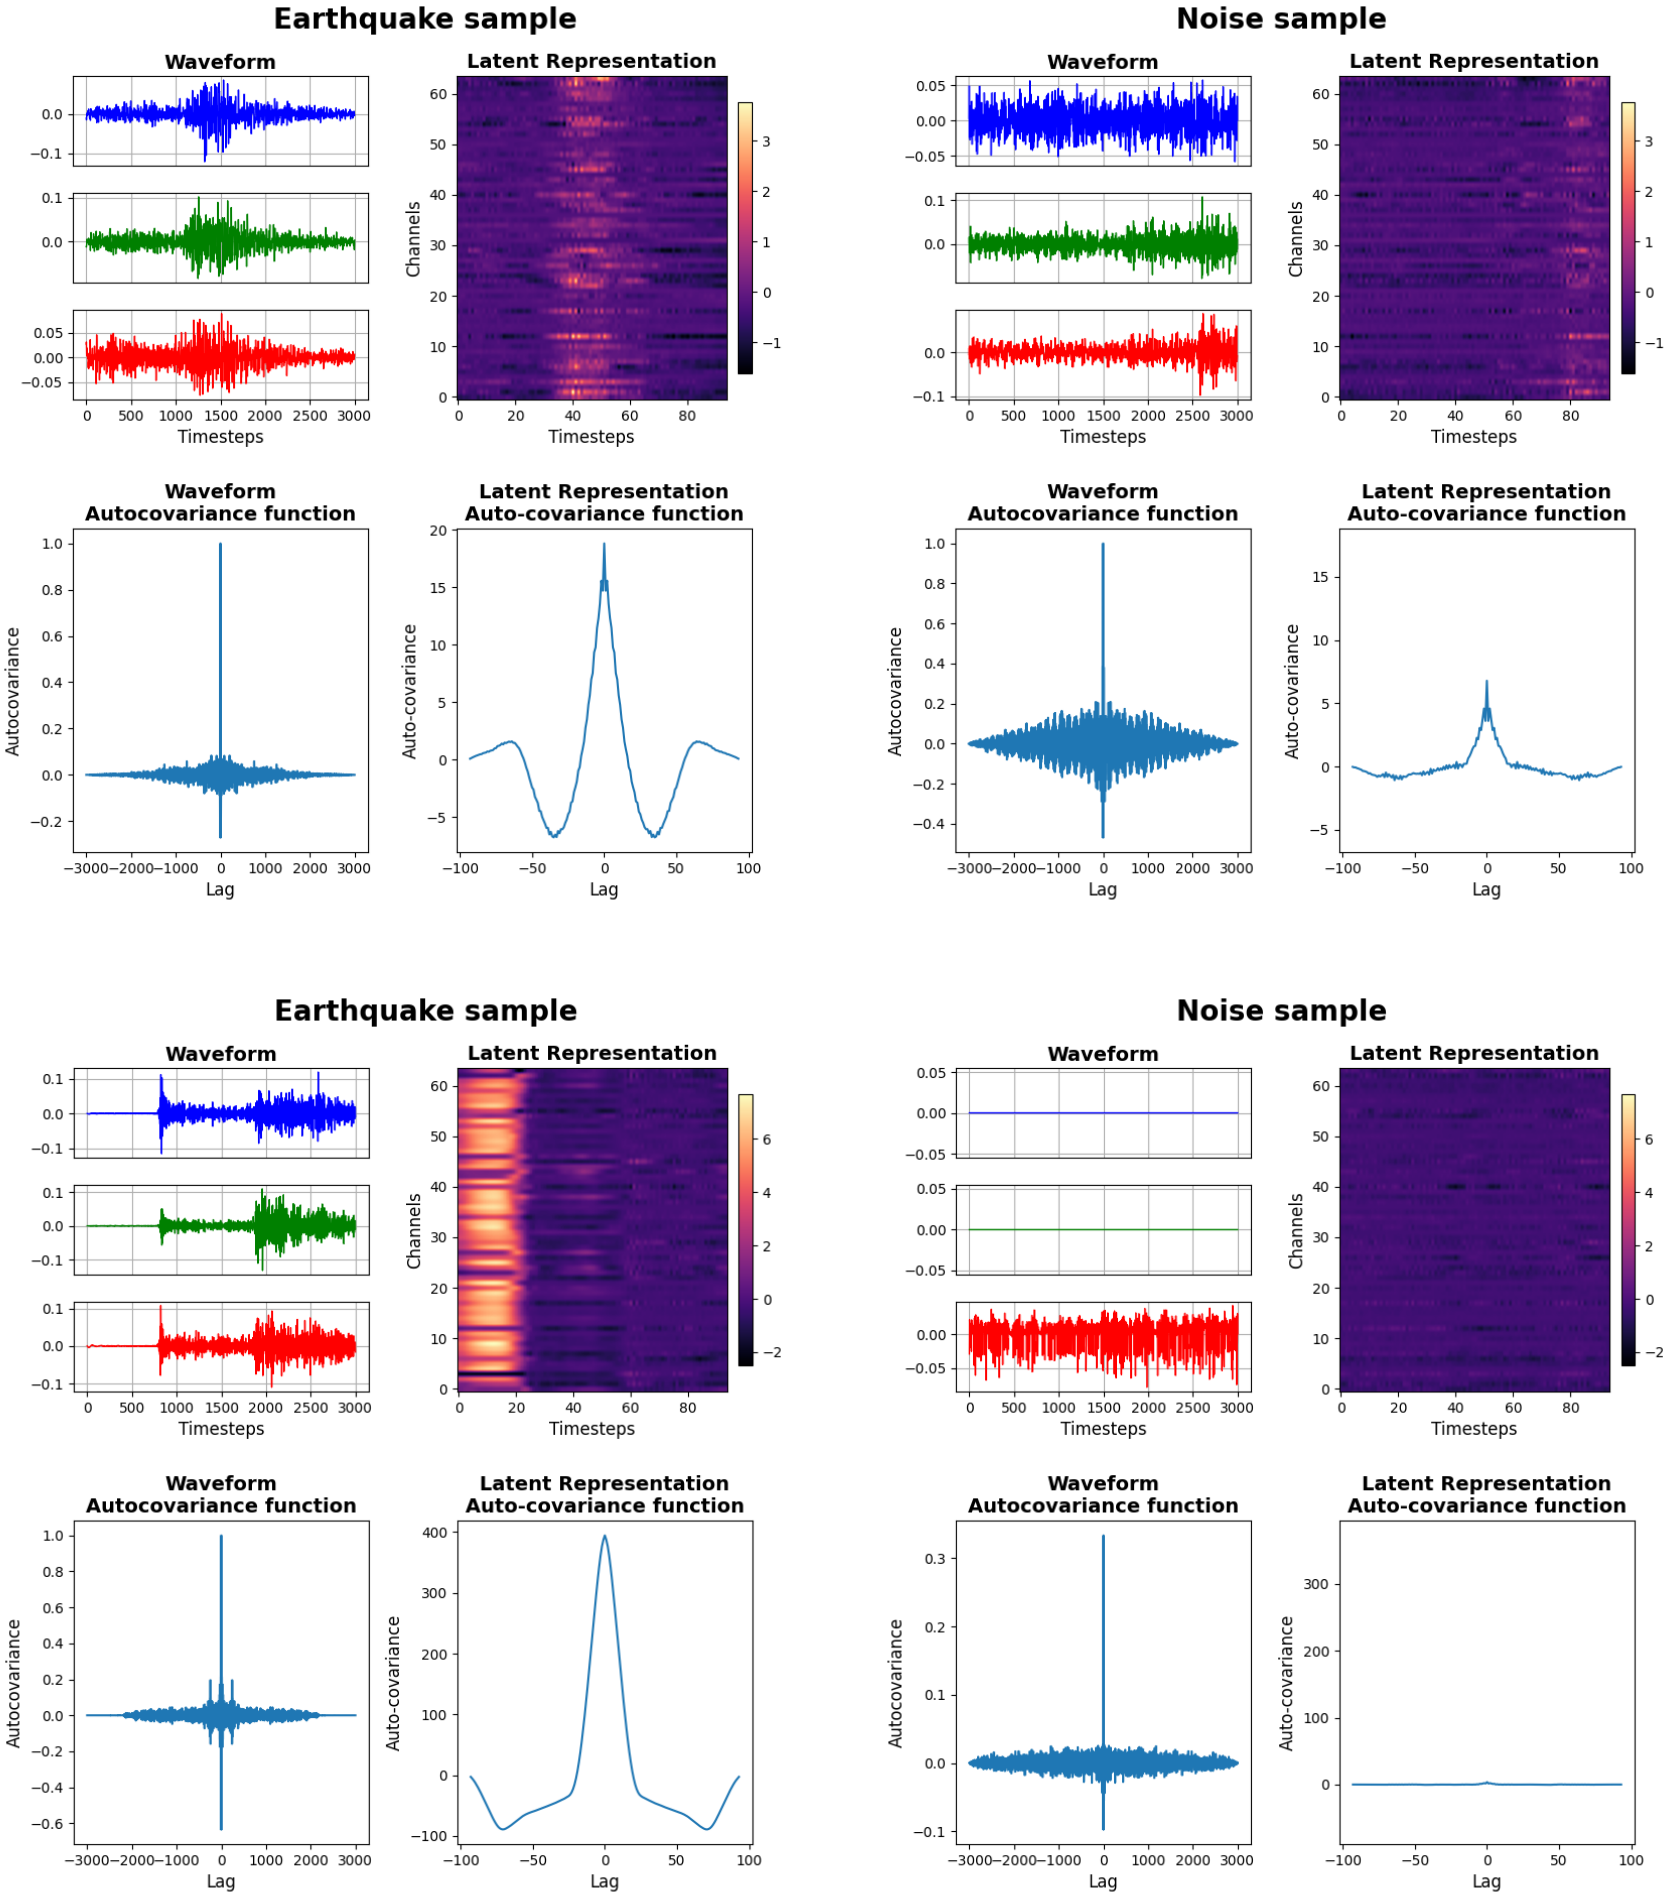}
    \caption{Samples for Single autoencoder method. Earthquake signals, representations, and covariances of earthquake signals and representations are given in the left-most two columns while right-most two columns involve visuals related to noise signals.}
    \label{fig:autcovariance_samples}
\end{figure}

\begin{figure}[t]
    \centering
    \setfigurenum{S4}
    \noindent\includegraphics[width=\linewidth]{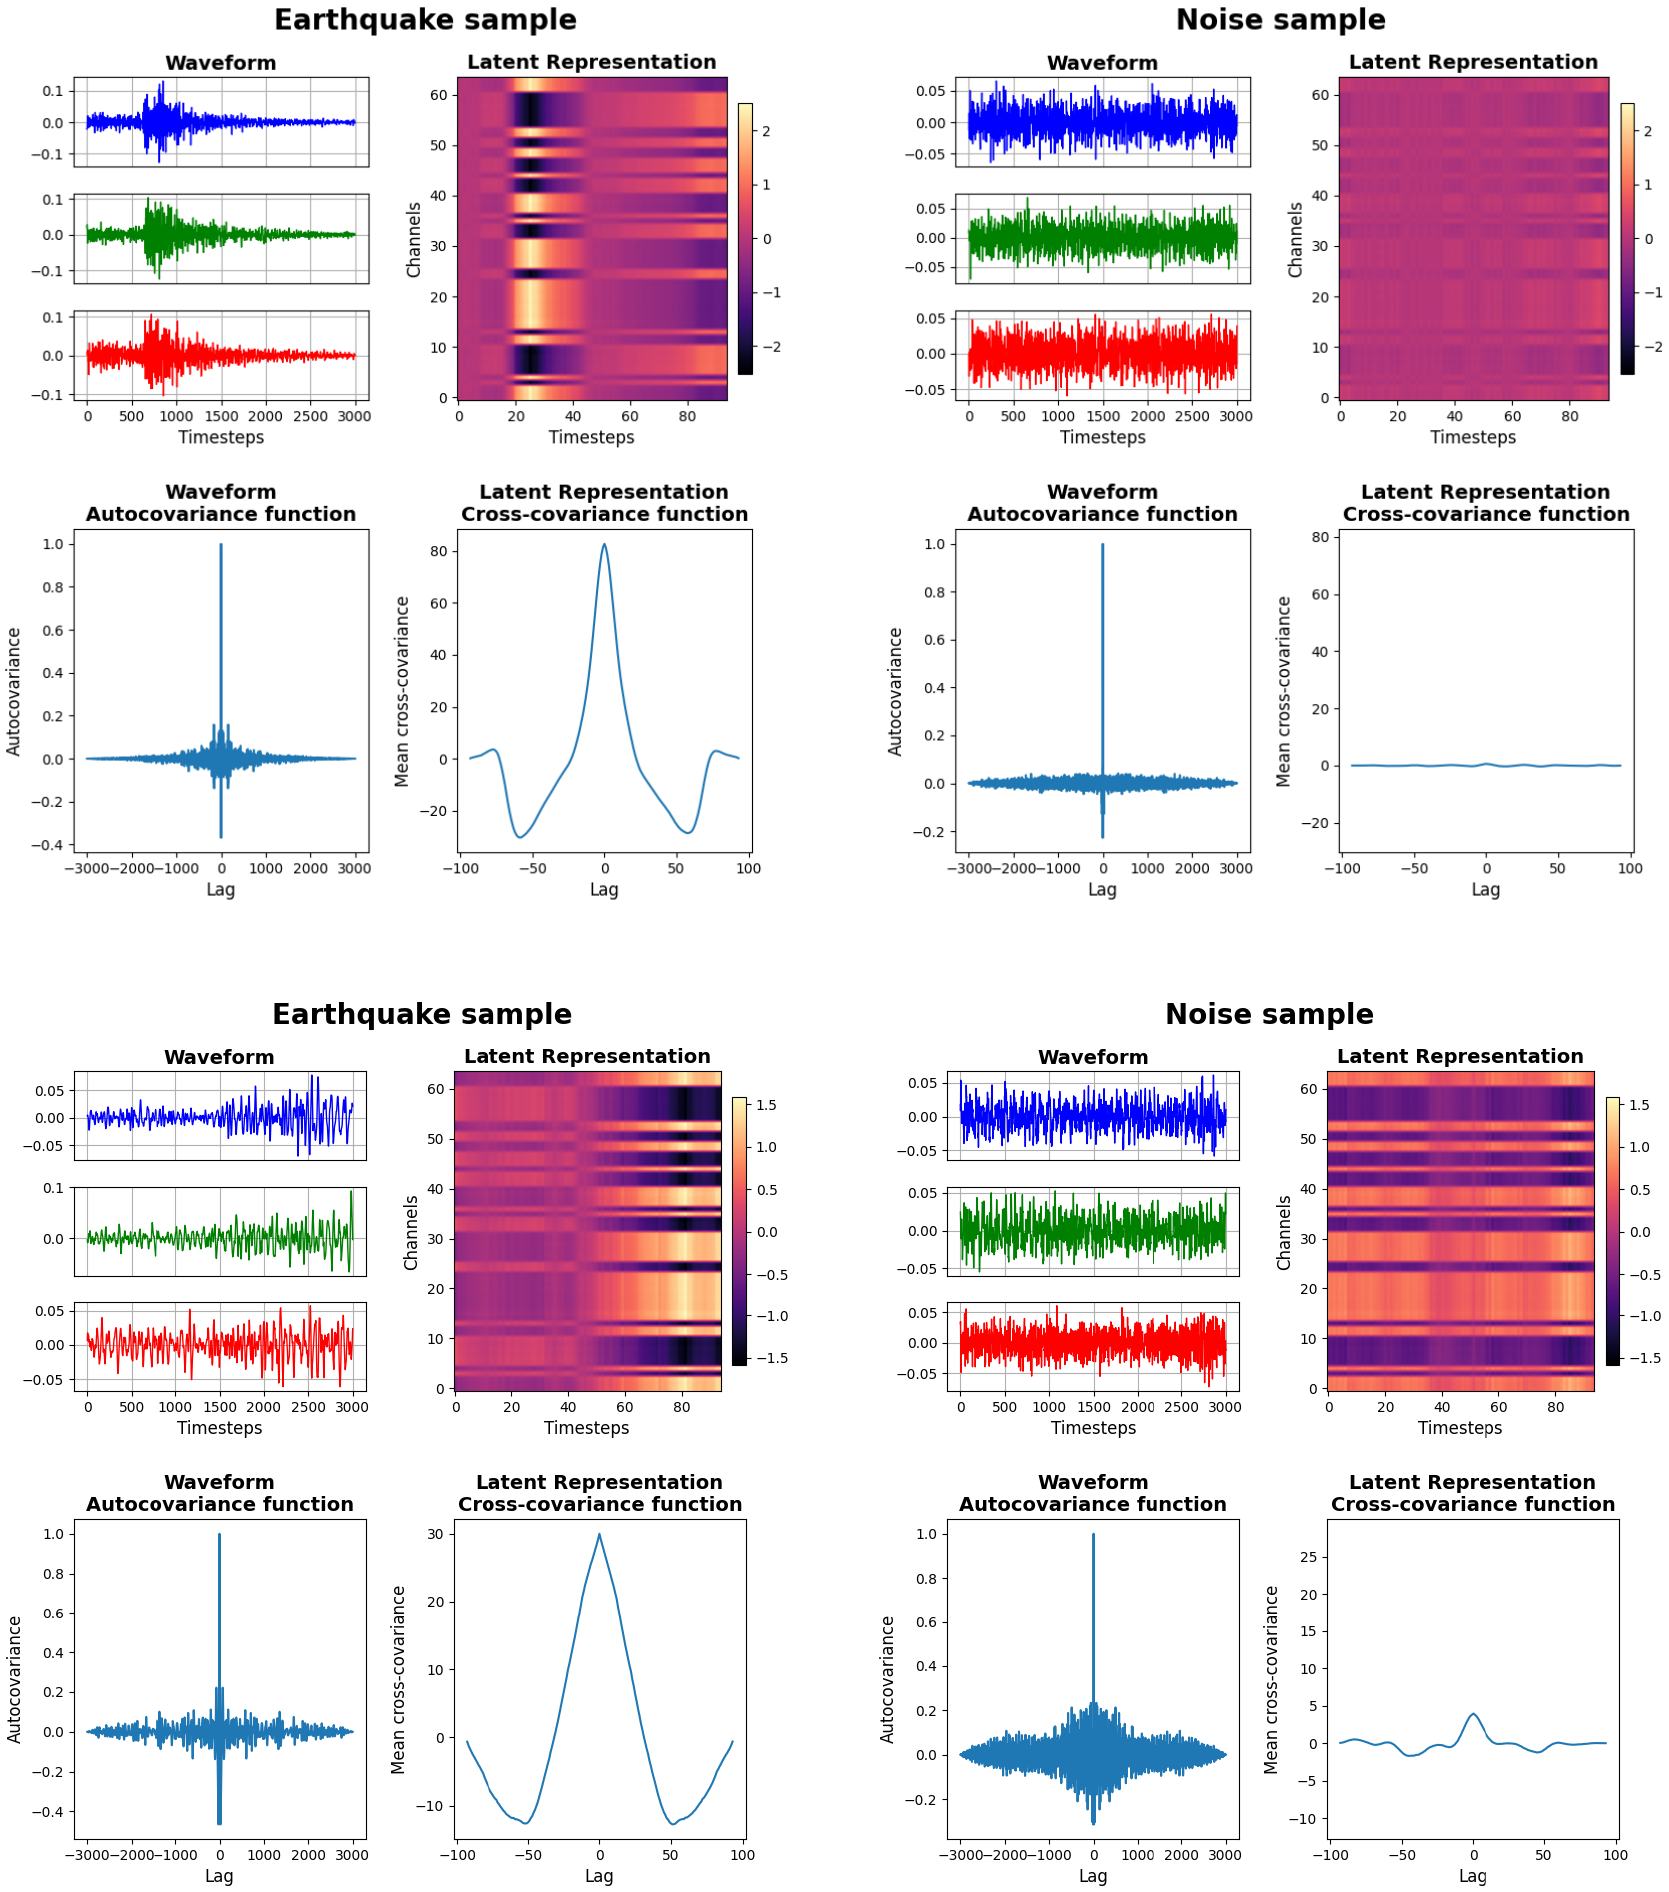}
    \caption{Samples for Multiple autoencoders method. Earthquake signals, representations, and covariances of earthquake signals and representations are given in the left-most two columns while right-most two columns involve visuals related to noise signals.}
    \label{fig:representation_cross_covariances_samples}
\end{figure}

\end{document}
